# Supplementary material for: RIP Twitter API: A eulogy to its vast research contributions
Source: arXiv:2404.07340 source file (2025-10-13)
Supplement: Supplementary file 2 [file S4_Appendix.pdf]

\*Taken from Final\_Dataset\_Dec2023 at  
[github.com/ryanmurt/Twitter](https://github.com/ryanmurt/Twitter), (bottom of Top Disc by Most Cited tab)

### **Topics taken from the 5 most cited studies from each discipline:**

The spread of true vs false news

Factors contributing to the spread of content on Twitter

The practice of retweeting on Twitter

How do ideological preferences impact the exchange of information?

How do emotions impact retweets? Info diffusion

Identifying influential users on Twitter

automatic methods for assessing the credibility of tweets.

Using Twitter to follow and analyze public attention (ie. During a pandemic)

Analyzing privacy in social media.

What causes certain content to be retweeted more than others?

Strategies for tracking health concerns, outbreaks, understanding health information disparities in communities

Studying misuse and misunderstanding of the use of antibiotics

A study of how twitter data is used in health research.

Studying the marketing and promotion of an e-cigarette from a public health perspective

Using Twitter to identify influenza outbreaks faster

Efficacy of conducting psychological tests online

Using twitter to identify diurnal and seasonal mood rhythms across the world

Efficacy of conducting psychological tests online

Using tweets to understand consumer sentiment toward brands.

Proposes a way of classifying tweet content to mitigate user overwhelm from too much content

Using geospatial data from twitter to identify and track events such as earthquakes

Understanding how social media can be used in higher education settings. A review of the literature.

A general study of what twitter is, how and why people use it.

Strategy for geolocating users based on tweet content

A new strategy for topic-modeling. How to train the topic model to a specific dataset and achieve more accurate topics.

What new technologies need to be developed to support the field of genomics?

Strategy for sentiment analysis

Comparing twitter, FB and Youtube for understanding and influencing consumer brand communication. Preferences?

Text mining strategy for analyzing customer sentiments about 3 pizza chains

Understanding how social media impacts effectuation

Strategy for text mining consumer sentiments toward specific brands

Research about how social media can be used to support the supply chain management field: practices, networking, stakeholder engagement, demand shaping, product development

Strategies for using AI in sentiment/opinion analysis

Using AI to identify fake news on social media..a specific framework

Using AI for sentiment analysis

Using sentiment analysis to help business organizations gain business insight into consumer opinions

Strategy for using AI in sentiment analysis of tweets.

**Most common topics:**

How information spreads on social media (ie. True vs fake news, factors contributing to retweeting/spread

How does ideology impact spread?

Identifying influential users, methods for assessing credibility of tweets,

Identifying and analyzing major events (pandemic, earthquake, influenza,

Studying behavior such as misuse and misunderstanding of antibiotics, the marketing/promotion of consumer products

Studying moods cross culturally (diurnal and seasonal)
